# Supplementary material for: Large Deviations for Accelerating Neural Networks Training
Source: arXiv:2303.00954 source file (2023-03-02)
Supplement: Supplementary file 1 [file suppli.tex]

\documentclass[sigconf,authordraft]{acmart}

\usepackage[ruled,vlined]{algorithm2e}
\usepackage{subcaption}
\usepackage[font=small,labelfont=bf]{caption}

\AtBeginDocument{%
  \providecommand\BibTeX{{%
    \normalfont B\kern-0.5em{\scshape i\kern-0.25em b}\kern-0.8em\TeX}}}

\setcopyright{acmcopyright}
\copyrightyear{2021}
\acmYear{2021}
\acmDOI{xx.xxxx/xxxxxxx.xxxxxxx}

%% These commands are for a PROCEEDINGS abstract or paper.
\acmConference[KDD '21]{KDD '21: ACM SIGKDD Conference on Knowledge and Data Discovery, June 03--05, 2021, Singapore}
\acmPrice{15.00}
\acmISBN{XXX-X-XXXX-XXXX-X/XX/XX}

\begin{document}

\title{Supplementary Section}
\section{LDP Background}
Some of the properties of the rate function are given by Varadhan's Lemma and Bryc's Lemma. 
\begin{theorem}{Varadhan's Lemma }
    If $\{\mu_\epsilon\}_{\epsilon>0}$ satisfies the LDP on $\mathcal{X}$ with rate function $\mathcal{I}$ then, 
\begin{equation}
\begin{aligned}
    lim_{\epsilon\to 0} \epsilon log \int_{\mathcal{I}}e^{F(x)/\epsilon}\mu_\epsilon(dx)=\Lambda_F\quad \forall F\in \mathrm{C}_b(\mathcal{X})
\end{aligned}    
\end{equation}
where $\mathrm{C}_b(\mathcal{X})$ is the space of continuous bounded functions on $\mathcal{X}$ and

\begin{equation}
    \begin{aligned}
    \Lambda_F=sup_{x\in\mathcal{X}}\left[ F(x)-\mathcal{I}(x)\right]
    \end{aligned}
\end{equation}
\end{theorem}

\begin{theorem}{Bryc's Lemma}
Suppose $\{\mu_\epsilon\}_{\epsilon>0}$ is exponentially tight and the limit in Varadhan's lemma exits $\forall F\in \mathrm{C}_b(\mathcal{X})$. Then, $\{\mu_\epsilon\}_{\epsilon>0}$ satisfies LDP with rate function $\mathcal{I}$ given by
\begin{equation}
    \begin{aligned}
    \mathcal{I}(x)=sup_{F\in \mathrm{C}_b(\mathcal{X})}\left[F(x)-\Lambda_F \right]\quad x\in\mathcal{X}
    \end{aligned}
\end{equation}
\end{theorem}

\section{Performance on smaller datasets}
\begin{table}[htb]
  \centering
          \begin{tabular}{|l|c|c|c|}
            \toprule
            Name & $N$ & $d$ & $a$ \\
            \midrule
            Pima  &  768  &  8  &  34.896\% \\ 
            Wine  &  129  &  13  &  7.752\% \\ 
            Cardio  &  1831  &  21  &  9.612\% \\ 
            Pendigits  &  6870  &  16  &  2.271\% \\ 
            Thyroid  &  3772  &  6  &  2.466\% \\ 
            Vowels  &  1456  &  12  &  3.434\% \\ 
            Breast cancer  &  683  &  9  &  34.993\% \\ 
            Lympho  &  148  &  18  &  4.054\% \\ 
            Annthyroid  &  7200  &  6  &  7.417\% \\ 
            WBC  &  378  &  30  &  5.556\% \\ 
            Mammography  &  11183  &  6  &  2.325\% \\ 
            Glass  &  214  &  9  &  4.206\% \\ 
            Cover  &  286048  &  10  &  0.96\% \\ 
            Vertebral  &  240  &  6  &  12.5\% \\ 
            % breast-cancer-unsupervised-ad.csv  &  367  &  30  &  30    2.725\% \\ 
            % Pen-global-unsupervised-ad.csv  &  809  &  16  &  16    11.125\% \\ 
          \bottomrule
            % \caption{}
        \end{tabular}
    \caption{Description of the benchmark data sets used for evaluation of the anomaly detection ({\em source}: Outlier Detection DataSets /ODDS~\citep{Rayana:2016}) capabilities of the proposed model. $N$ - number of instances, $d$ - number of attributes, and $a$ - fraction of known anomalies in the data set.}
    \label{tab:datadescription}
\end{table}

\begin{table*}
    \caption{Comparing LAD with existing anomaly detection algorithms using ROC-AUC as the evaluation metric.}  
    \label{tab:auc_small}
  \begin{tabular}{|l|c|c|c|c|c|c|c|c|}
    \toprule
    Data & LOF & KMeans-- & KNN & OCSVM & iForest & EE & LAD \\
    \midrule
    PIMA & 0.59 & 0.64 & 0.64 & 0.52 & 0.62 & 0.62 & 0.68  \\
    VERTEBRAL & 0.51 & 0.43 & 0.36 & 0.61 & 0.45 & 0.43 & 0.35  \\
    THYROID & 0.62 & 0.56 & 0.95 & 0.51 & 0.77 & 0.82 & 0.92  \\
    WBC & 0.95 & 0.8 & 0.94 & 0.47 & 0.8 & 0.7 & 0.95 \\
    CARDIO & 0.59 & 0.81 & 0.87 & 0.57 & 0.76 & 0.71 & 0.96  \\
    MAMMOGRAPHY & 0.74 & 0.63 & 0.85 & 0.55 & 0.6 & 0.49 & 0.87  \\
    GLASS & 0.72 & 0.54 & 0.87 & 0.73 & 0.54 & 0.48 & 0.73  \\
    BREASTW & 0.35 & 0.23 & 0.99 & 0.81 & 0.95 & 0.95 & 0.96  \\
    VOWELS & 0.89 & 0.58 & 0.81 & 0.64 & 0.6 & 0.51 & 0.77  \\
    PENDIGITS & 0.54 & 0.59 & 0.74 & 0.51 & 0.71 & 0.54 & 0.91 \\
    \midrule
    AVERAGE RANK & 4.75 & 5.6 & 2.85 & 6.2 & 5.1 & 6.2 & 2.7 \\
  \bottomrule

\end{tabular}
\end{table*}

\bibliographystyle{ACM-Reference-Format}
% \bibliography{Bib/bibliography}    
\bibliography{Bib/bibliography,Bib/bibliography_ts,Bib/bibliography_covid,Bib/bibliography_ldp,Bib/bibliography_hd}
\end{document}
