# Supplementary material for: Large Deviations for Accelerating Neural Networks Training
Source: arXiv:2303.00954 source file (2023-03-02)
Supplement: Supplementary file 2 [file appendix.tex]

\section{Performance on smaller datasets}
\begin{table}[htb]
  \centering
          \begin{tabular}{|l|c|c|c|}
            \toprule
            Name & $N$ & $d$ & $a$ \\
            \midrule
            Pima  &  768  &  8  &  34.896\% \\ 
            Wine  &  129  &  13  &  7.752\% \\ 
            Cardio  &  1831  &  21  &  9.612\% \\ 
            Pendigits  &  6870  &  16  &  2.271\% \\ 
            Thyroid  &  3772  &  6  &  2.466\% \\ 
            Vowels  &  1456  &  12  &  3.434\% \\ 
            Breast cancer  &  683  &  9  &  34.993\% \\ 
            Lympho  &  148  &  18  &  4.054\% \\ 
            Annthyroid  &  7200  &  6  &  7.417\% \\ 
            WBC  &  378  &  30  &  5.556\% \\ 
            Mammography  &  11183  &  6  &  2.325\% \\ 
            Glass  &  214  &  9  &  4.206\% \\ 
            Cover  &  286048  &  10  &  0.96\% \\ 
            Vertebral  &  240  &  6  &  12.5\% \\ 
            % breast-cancer-unsupervised-ad.csv  &  367  &  30  &  30    2.725\% \\ 
            % Pen-global-unsupervised-ad.csv  &  809  &  16  &  16    11.125\% \\ 
          \bottomrule
            % \caption{}
        \end{tabular}
    \caption{Description of the benchmark data sets used for evaluation of the anomaly detection ({\em source}: Outlier Detection DataSets /ODDS~\citep{Rayana:2016}) capabilities of the proposed model. $N$ - number of instances, $d$ - number of attributes, and $a$ - fraction of known anomalies in the data set.}
    \label{tab:datadescription}
\end{table}

\begin{table*}
    \caption{Comparing LAD with existing anomaly detection algorithms using ROC-AUC as the evaluation metric.}  
    \label{tab:auc_small}
  \begin{tabular}{|l|c|c|c|c|c|c|c|c|}
    \toprule
    Data & LOF & KMeans-- & KNN & OCSVM & iForest & EE & LAD \\
    \midrule
    PIMA & 0.59 & 0.64 & 0.64 & 0.52 & 0.62 & 0.62 & 0.68  \\
    VERTEBRAL & 0.51 & 0.43 & 0.36 & 0.61 & 0.45 & 0.43 & 0.35  \\
    THYROID & 0.62 & 0.56 & 0.95 & 0.51 & 0.77 & 0.82 & 0.92  \\
    WBC & 0.95 & 0.8 & 0.94 & 0.47 & 0.8 & 0.7 & 0.95 \\
    CARDIO & 0.59 & 0.81 & 0.87 & 0.57 & 0.76 & 0.71 & 0.96  \\
    MAMMOGRAPHY & 0.74 & 0.63 & 0.85 & 0.55 & 0.6 & 0.49 & 0.87  \\
    GLASS & 0.72 & 0.54 & 0.87 & 0.73 & 0.54 & 0.48 & 0.73  \\
    BREASTW & 0.35 & 0.23 & 0.99 & 0.81 & 0.95 & 0.95 & 0.96  \\
    VOWELS & 0.89 & 0.58 & 0.81 & 0.64 & 0.6 & 0.51 & 0.77  \\
    PENDIGITS & 0.54 & 0.59 & 0.74 & 0.51 & 0.71 & 0.54 & 0.91 \\
    \midrule
    AVERAGE RANK & 4.75 & 5.6 & 2.85 & 6.2 & 5.1 & 6.2 & 2.7 \\
  \bottomrule

\end{tabular}
\end{table*}
